# Supplementary material for: Deep or Simple Models for Semantic Tagging? It Depends on your Data [Experiments]
Source: arXiv:2007.05651 source file (2020-10-08)
Supplement: Supplementary file 1 [file appendix_more.tex]

\section*{Appendix\_More}
\subsection*{Efficiency Evaluation}
% train time for each dataset (small dataset, acceptable)
% test time for large dataset (unacceptable)

\begin{table}[!t]
\centering
\scalebox{0.8}{
\begin{tabular}{|l|l|l|l|l|l|l|}
\hline
        & \multicolumn{3}{l|}{Training} & \multicolumn{3}{l|}{Testing} \\ \hline
Dataset & BERT (s)  & ML (s)  & ratio   & BERT (s)  & ML (s)  & ratio  \\ \hline
SUGG    & 260.34    & 0.64    & 408.86  & 2.05      & 0.02    & 92.07  \\ \hline
HOTEL   & 188.64    & 0.37    & 503.08  & 5.14      & 0.04    & 119.31 \\ \hline
SENT    & 273.77    & 0.72    & 381.73  & 7.79      & 0.14    & 54.41  \\ \hline
PARA    & 168.18    & 0.62    & 269.62  & 4.90      & 0.08    & 60.51  \\ \hline
FUNNY   & 119434.97 & 2490.48 & 47.96   & 4936.71   & 193.18  & 25.56  \\ \hline
HOMO    & 244.07    & 0.12    & 1967.18 & 8.12      & 0.01    & 821.85 \\ \hline
HETER   & 359.38    & 0.10    & 3752.43 & 5.15      & 0.01    & 641.56 \\ \hline
TV      & 167.09    & 1.02    & 163.31  & 4.91      & 0.06    & 86.56  \\ \hline
BOOK    & 161013.00 & 3996.83 & 40.29   & 20694.25  & 128.77  & 160.71 \\ \hline
EVAL    & 242.25    & 0.53    & 459.40  & 8.14      & 0.07    & 108.96 \\ \hline
REQ     & 244.88    & 0.68    & 359.39  & 8.19      & 0.14    & 56.80  \\ \hline
FACT    & 244.08    & 0.55    & 444.29  & 8.17      & 0.14    & 56.89  \\ \hline
REF     & 243.42    & 0.59    & 412.68  & 8.23      & 0.13    & 61.46  \\ \hline
QUOTE   & 246.61    & 0.77    & 318.72  & 8.19      & 0.14    & 58.08  \\ \hline
ARGUE   & 673.70    & 1.99    & 339.26  & 18.19     & 0.33    & 55.93  \\ \hline
SUPPORT & 549.61    & 1.81    & 304.08  & 17.51     & 0.32    & 54.61  \\ \hline
AGAINST & 550.64    & 1.81    & 304.97  & 17.48     & 0.43    & 40.37  \\ \hline
AMAZON  & 12085.75  & 199.71  & 60.52   & 43.85     & 1.55    & 28.36  \\ \hline
YELP    & 12628.28  & 334.39  & 37.76   & 54.90     & 15.70   & 3.50   \\ \hline
\end{tabular}
}
\caption{F1 gain of BERT (improvement over 10 percent are marked in red)}
\label{table:bert_price}
\end{table}   

We divided our datasets into two categories, i.e. small and large according to their sizes. FUNNY, BOOK, AMAZON and YELP belong to large datasets as they contain more than 500,000 data records. The others datasets belong to the small category as the size of each dataset is smaller than 3, 000. We calculated training time and prediction time for each of LR, SVM and BERT. We showed the results at Table~\ref{table:bert_price}. 

% training time
BERT consumes a lot computation power for both training and testing. Even we used GPU for BERT, It still took significant amount of time than the CPU only method LR and SVM. On small datasets, the cost can be hundreds or even thousands times more expensive. However, the exact training time is usually hundreds of seconds and still acceptable. This is because the scale of a dataset is small so the latency is acceptable. On large datasets, the cost for BERT is tens of times more expensive and smaller than the number for small datasets. This is because a large dataset has larger vocabulary, so a data record is projected to a higher dimension for LR and SVM. Although the magnitude looks small, the exact training time is large. BOOK took the longest training time which is about 5 days. Large training overhead will be a big problem in practice for model debugging and deployment, which usually run model training multiple times.  

Testing time shows similar pattern. BERT show significant more training time than LR and SVM on small datasets. This is because BERT model is large so initialization takes long time. But the loading cost can be amortized when the dataset is large. Prediction on 20\% BOOK takes about 5 hours, which is acceptable. Considering BERT's improvement on large datasets are marginal, it is really a question that whether it is worth to use BERT for large datasets. 

Overall, using LR and SVM are the two most economical methods for large datasets. Both training and testing are agile, and there are huge space for improvement as both models are small and easy to tune. Considering today GPU resource costs even more than CPU resources (e.g. Amazon AWS allows free use of a CPU server but charges for a GPU server), using BERT for large datasets may not be a good choice.

\subsection{*Quality evaluation}

\begin{table}[!t]
\centering
\scalebox{1}{
\centering
\begin{tabular}{|l|l|l|l|l|l|}
\toprule
Dataset & LR            & SVM           & CNN  & LSTM & BERT          \\ \midrule
SUGG    & 0.79          & 0.77          & 0.77 & 0.68 & \textbf{0.86} \\ 
HOTEL   & 0.53          & 0.55          & 0.46 & 0.59 & \textbf{0.67} \\ 
SENT    & 0.50          & 0.51          & 0.43 & 0.45 & \textbf{0.57} \\ 
PARA    & 0.56          & 0.59          & 0.50 & 0.48 & \textbf{0.65} \\ 
FUNNY   & 0.29          & \textbf{0.38} & 0.08 & 0.12 & 0.32          \\ 
HOMO    & 0.87          & 0.89          & 0.90 & 0.90 & \textbf{0.95} \\ 
HETER   & 0.87          & 0.87          & 0.87 & 0.86 & \textbf{0.93} \\ 
TV      & 0.70          & 0.68          & 0.54 & 0.63 & \textbf{0.81} \\ 
BOOK    & \textbf{0.17} & 0.15          & 0.06 & 0.11 & 0.15          \\ 
EVAL    & 0.72          & 0.73          & 0.75 & 0.73 & \textbf{0.81} \\ 
REQ     & 0.69          & 0.69          & 0.67 & 0.70 & \textbf{0.84} \\ 
FACT    & 0.69          & 0.69          & 0.74 & 0.73 & \textbf{0.82} \\ 
REF     & 0.80          & 0.79          & 0.78 & 0.83 & \textbf{0.93} \\ 
QUOTE   & 0.10          & 0.10          & 0.14 & 0.58 & \textbf{0.66} \\ 
ARGUE   & 0.72          & 0.72          & 0.70 & 0.72 & \textbf{0.78} \\ 
SUPPORT & 0.46          & 0.45          & 0.41 & 0.41 & \textbf{0.54} \\ 
AGAINST & 0.53          & 0.51          & 0.41 & 0.43 & \textbf{0.62} \\ 
AMAZON  & 0.93          & 0.93          & 0.89 & 0.86 & \textbf{0.96} \\ 
YELP    & 0.94          & \textbf{0.96} & 0.94 & 0.93 & \textbf{0.96} \\ 
FUNNY*  & 0.81          & 0.81          & 0.68 & 0.73 & \textbf{0.82} \\ 
BOOK*   & 0.72          & 0.7           & 0.70 & 0.67 & \textbf{0.74} \\ \bottomrule
\end{tabular}
}
\caption{F1 of all models (best results marked in bold) \yuliang{1. add a row of average sccore 2. move to appendix if out of space 3. group the datasets}}
\label{table:f1_all_model}
\end{table}

\begin{table*}[!t]
\begin{tabular}{|l|l|l|l|l|l|l|l|l|}
\hline
                      &             &                      & \multicolumn{3}{l|}{Feature Representation} & \multicolumn{3}{l|}{Weighting} \\ \hline
paper                  & apps        & base model           & BoW   & Embedding   & domain-specific   & IDF   & Attention  & Sequence  \\ \hline
\cite{NegiB15emnlp}         & suggestion  & SVM                  & T                 &               & T       &       &            &           \\ \hline
\cite{semeval19liuWY}       & suggestion  & BERT                 &                   & T             &         &       & T          &           \\ \hline
\cite{GuyMNR17www}          & tip         & LR                   & T                 & T             & T       & T     &            &           \\ \hline
\cite{WicaksonoM13cikm}     & suggestion  & CRF                  & T                 &               & T       & T     &            &           \\ \hline
\cite{NegiAMB16starsem}     & suggestion  & LSTM                 &                   & T             &         &       &            & T         \\ \hline
\cite{KimH06acl}            & argument    & Max Entropy          & T                 &               & T       &       &            &           \\ \hline
\cite{ParkJM10acl}          & tip         & SVM                  & T                 &               &         &       &            &           \\ \hline
\cite{spoiler19acl}         & spoiler     & HAN                  &                   & T             & T       &       & T          &           \\ \hline
\cite{NovgorodovEGR19www}   & description & LSTM                 &                   & T             &         &       &            & T         \\ \hline
\cite{WeberUG12wsdm}        & tip         & SVM                  & T                 & T             & T       &       &            &           \\ \hline
\cite{HuaNBW19naacl}        & argument    & BiLSTM, CRF          &                   & T             & T       &       &            & T         \\ \hline
\cite{MoralesZ17emnlp}      & humor       & AdaBoost             & T                 & T             & T       &       &            &           \\ \hline
\cite{ZouL19naacl}          & humor       & BiLSTM, CRF          &                   &               &         &       &            &           \\ \hline
\cite{StabMSRG18emnlp}      & argument    & CNN + biLSTM         &                   &               &         &       &            &           \\ \hline
\cite{DiaoL0FWZX19www}      & humor       & CNN, LSTM, Attention &                   &               &         &       &            &           \\ \hline
\cite{Boyd-GraberGZ13asist} & spoiler     & SVM                  &                   &               &         &       &            &           \\ \hline
\end{tabular}
\caption{Extraction algorithm design choice}
\label{table:designchoice}
\end{table*}
